# Supplementary material for: ClarQ-LLM: A Benchmark for Models Clarifying and Requesting Information in Task-Oriented Dialog
Source: arXiv:2409.06097 source file (2024-09-14)
Supplement: Supplementary file 1 [file cq-and-info-seeking.tex]

\section{Clarification Question and Information-Seeking Question}
\label{sec:Clarification Question or Information-Seeking Question}

ClarQ-LLM allows seekers to obtain the information they need through either clarification questions or information-seeking questions. 
For example, the specific clarification question from seeker S1 in Figure~\ref{figure:conv}, `Which type of pizza would you like? Pepperoni or Breakfast Pizza?' can be broadened to an information-seeking question: `What type of pizza would you like?'
However, this does not mean that ClarQ-LLM is completely aligned with traditional information-seeking tasks. 
Taking RiSAWOZ~\cite{quan-etal-2020-risawoz} as an example, this dataset lists all the desired information at the start of the task and requires the seeker to obtain each piece of information by asking questions. 
In contrast, ClarQ-LLM does not explicitly list the specific information that seekers need to obtain. 
Instead, it requires seekers to identify uncertainties in the conversation and ask further questions based on these.
For instance, in the dialogue task in Figure~\ref{figure:conv}, whether the seeker needs to inquire about the pizza size, type, and type of bread depends on their own analysis. 
If the restaurant offers only one type of pizza and garlic bread, then there would be no need for further questions.
