# Supplementary material for: ClarQ-LLM: A Benchmark for Models Clarifying and Requesting Information in Task-Oriented Dialog
Source: arXiv:2409.06097 source file (2024-09-14)
Supplement: Supplementary file 2 [file Dataset-Statistics.tex]

\section{Extra Details of the Dataset}
\label{sec:Extra Details of the Dataset}

\subsection{Dataset Statistics}
\label{sec:Dataset Statistics}
ClarQ-LLM dataset features 31 types of tasks. 
Each type consists of 10 specific tasks, with each one having its own unique game background and conversation. 
We've organized these 31 types into two main groups: 26 for testing, to evaluate how well seekers perform, and 5 for development, aimed at building and testing applications. 
ClarQ-LLM doesn't include a training set.

Regarding the game environment, our dataset includes a diverse range of 393 items, 321 different skills or actions, and 732 unique scenes. 
For the quantity of uncertainty, our dataset encompasses a variety of setups: 1 task comes with 2 uncertainties, 52 tasks with 3 uncertainties, 125 tasks with 4 uncertainties, 92 tasks with 5 uncertainties, and 38 tasks with 6 uncertainties. 
In terms of structural complexity, as measured by the depth of provider response trees, our dataset includes 165 tasks structured within trees of depth 1, 129 tasks structured within trees of depth 2, 14 tasks structured within trees of depth 3, and only 2 tasks that feature the most complex structures within trees of depth 4.

\subsection{Construction Principles}
The database we constructed follows three basic principles to ensure dataset quality and usability.

\paragraph{Question types.}
% Our study aims to facilitate the development of an conversational agent whose performance is comparable to that of the human player depicted in Figure~\ref{figure:conv-2}.

While there are various causes and types of clarification question \citep[see e.g.][]{rodriguez-schlangen-2004-form,rieser-moore-2005-implications,purver-etal-2001-means}, our dataset's primary objective is to determine if the model can effectively ask relevant questions about ambiguous references. 
However, merely asking these clarification questions does not suffice to gather all the necessary information for completing a task. 
Therefore, we also expect the seeker to ask information-seeking questions to accomplish the task, as discussed in detail in Appendix~\ref{sec:Clarification Question or Information-Seeking Question}.% as illustrated in subdialogue 4 of Figure~\ref{figure:conv-2}.

\paragraph{Talking in a Virtual Game World.}
We carry out our dialogue tasks in different virtual game worlds that we've designed with a lot of care. 
These worlds might have magical elements, like casting spells or fighting monsters.
Even though these tasks happen in a game setting, some of them are closely linked to real-life skills. 
For instance, tasks related to electronic engineering require the player to have knowledge of electronic parts. This approach tests whether the model can adapt to entirely new tasks and possess specific real-world knowledge.

\paragraph{Following Ethical Rules.}

When creating our database, we're very careful about ethics, avoiding any content that could lead to ethical issues. For example, we use fictional monsters instead of involving tasks that could harm people or animals. Likewise, for cooking tasks, we opt for vegetarian options to prevent harming animals.

% \paragraph{Keeping Things Logical and Clear.}

% In designing the database, we prioritize logical organization and clarity of information. 
% % Our dataset exclusively comprises the helper's responses, omitting the player's questions. 
% Consequently, we meticulously review the helper's responses to guarantee that players can intuitively discern the questions they ought to ask, based on both the task's background and the helper's guidance. 
% Essentially, the formulation of the helper's responses implicitly shapes the potential queries of the player. 
% For an in-depth explanation of how this process is implemented, please refer to Section~\ref{sec:Predefined-Helper-Responses}.

\subsection{Annotation Steps}

We develop our dataset in five steps, involving around 700 hours of human labor in total:

Step 1: Creating Initial Dialogues Between the Seeker and Provider. We assembled a team consisting of four college students tasked with writing the dialogues in Chinese. The diverse composition of the team contributed to a greater variety of tasks.

Step 2: Improving the Drafts. After completing the initial versions, we identified many errors and illogical parts. A post-doctoral researcher meticulously reviewed each task to correct any issues, ensuring that everything was logical and adhered to the principles of data annotation. Simultaneously, he annotated the provider's responses into a tree.

Step 3: Reviewing the Chinese Version. Next, another undergraduate checked the Chinese data for anything that might be missing or unclear, didn't make sense, contained typos, or whether the provider response tree was correctly organized.

Step 4: Translation and Cultural Adaptation. After finalizing the Chinese version, we utilized GPT-4 to translate it into English. A bilingual student reviewed the translation to correct any inaccuracies. Then, a PhD student, who is a native English speaker, evaluated the dialogues to ensure they were clear, logical, and consistent with Western cultural expectations.

Step 5: Testing with Real Conversations. Once everything was reviewed and fixed, we asked some students who hadn’t seen the data before to talk with the provider agent model. This was to see how well the model worked and if the way we organized the provider's responses were right. After these tests, we had our final dataset.

\subsection{Introduction to Task Types}
\label{sec:Introduction to Task Types}
Here is an introduction to 31 different types of tasks:

\begin{enumerate}[label=\arabic*.]
    \item \textbf{Gather Resources}: This type of task requires seeker to collect specific resources.
    \item \textbf{Escort Mission}: In these tasks, seekers must successfully escort a specific target to a designated location.
    \item \textbf{Stealth Mission}: Seekers act as agents to retrieve specific documents or items.
    \item \textbf{Survival Challenge}: Seekers must survive within the game environment.
    \item \textbf{Construction Task}: These tasks require seekers to build specific structures, such as shelters.
    \item \textbf{Defense Mission}: Seekers must defend against enemy attacks.
    \item \textbf{Competition}: Seekers need to win in specific competitions.
    \item \textbf{Weapon Manufacturing}: This task involves seekers creating specific weapons.
    \item \textbf{Hunting Expedition}: Seekers must hunt specific creatures.
    \item \textbf{Rescue Mission}: Seekers are tasked with rescuing specific individuals.
    \item \textbf{Arena Battle}: Seekers must defeat specific enemies in the arena.
    \item \textbf{Scientific Experiment}: Seekers act as scientists to complete specific experiments.
    \item \textbf{Photography Mission}: Seekers must take photos of specific scenes or characters, requiring basic photography skills.
    \item \textbf{Trade Task}: Seekers must complete trades with specific characters.
    \item \textbf{Exploration Journey}: These tasks require seekers to explore specific areas.
    \item \textbf{Electrical Engineering}: Seekers need basic knowledge of electrical engineering to develop or repair related products.
    \item \textbf{Automobile Manufacturing}: Seekers assemble vehicles, requiring basic vehicle knowledge.
    \item \textbf{Painting Task}: Seekers paint specific images at designated locations, using their painting skills.
    \item \textbf{Repair Mission}: Seekers repair specific items by replacing parts.
    \item \textbf{Training Session}: Seekers train specific targets, such as teaching subordinates the fireball magic skill.
    \item \textbf{Digging Mission}: Seekers dig in specific areas or for specific items, such as digging a trap.
    \item \textbf{Electronic Engineering}: Seekers need knowledge of electrical engineering to complete specific grid setups.
    \item \textbf{Planting Task}: Seekers successfully plant specific plants.
    \item \textbf{Alliance Building}: Seekers complete tasks to form alliances with others.
    \item \textbf{Cooking Delicacies}: Seekers cook specific dishes.
    \item \textbf{Video Production}: Seekers produce specific videos.
    \item \textbf{Animal Care}: Seekers take care of specific animals.
    \item \textbf{Archaeological Excavation}: Seekers complete the excavation and exploration of ancient ruins.
    \item \textbf{Escape Mission}: Seekers must escape from designated locations.
    \item \textbf{Planning Tourism}: Seekers plan trips, including booking hotels.
    \item \textbf{Magic Task}: These tasks involve fictional magic, requiring seekers to learn specific spells.
\end{enumerate}
