# Supplementary material for: ClarQ-LLM: A Benchmark for Models Clarifying and Requesting Information in Task-Oriented Dialog
Source: arXiv:2409.06097 source file (2024-09-14)
Supplement: Supplementary file 3 [file hp.tex]

\section{Model Inference Parameters}
\label{sec:Hyperparameters}   

For the GPT series, we access the GPT models using the `chat.completions.create' method from the OpenAI library. The main parameters for this method include the model name, temperature and seed. The model names are `gpt-4o-2024-05-13', `gpt-4-0613' and `gpt-3.5-turbo-0613,' corresponding to GPT-4o, GPT-4 and GPT-3.5, respectively. The value for `temperature' is always set to 0, and for `seed' is always set to 8848.

For ERNIE-Bot-4 model,  we access it using the `chat\_comp.do' method from the qianfan library. The main parameters for this method include the model name and temperature. The model name is `ERNIE-Bot-4'. The value for `temperature' is always set to 0.0000001.

For LLAMA2, we adhered to a consistent set of parameters to maintain uniformity in the outcomes. Below, we enumerate the parameters applied across our model runs:

\begin{itemize}[noitemsep]
  \item \texttt{do\_sample}: True
  \item \texttt{top\_p}: 1.0
  \item \texttt{temperature}: 1.0
  \item \texttt{min\_length}: None 
  \item \texttt{use\_cache}: True
  \item \texttt{top\_k}: 50
  \item \texttt{repetition\_penalty}: 1.0
  \item \texttt{length\_penalty}: 1
\end{itemize}

Consequently, we standardized the seed setting in our computational environment, leveraging Torch's seed configuration capabilities:

\begin{verbatim}
torch.cuda.manual_seed(8848)
torch.manual_seed(8848)
\end{verbatim}

This approach was instrumental in preserving the consistency of experimental conditions.
